# Supplementary material for: Computing Delay-Constrained Least-Cost Paths for Segment Routing is Easier Than You Think
Source: arXiv:2011.05191 source file (2020-11-10)
Supplement: Supplementary file 1 [file appendix.tex]

% \section{Notations}
% \begin{table}[H]
% \caption{Notations used through the paper}
% \label{tab:notation}
% \begin{center}
% \begin{tabular}{ll}
% \toprule
% $G = (V,E)$ & Multi-graph $G$ with $(V,E)$ vertices, edges \\
% $G' = (V,E')$ & Transformed SR Graph\\
% $E(u,v)$ & Set of edges between $u$ and $v$ \\
% $M0, M1, M2$ & The three metrics (\#seg, IGP cost, delay))\\
% $c0, c1, c2$ & Constraints on each metric\\
% $dj_G(P)$ & The distance of the path $P$ in $G$ for metric $j$ \\
% $wj_G(l)$ & The weight of the link $l \in E$ for metric $j$ \\
% $P_G(u,v)$ & Best path regarding the M1 distance \\
% 	& from u to v \\
% % $sl(n)$ & Segment list towards the node n\\
% % $R_G(sl(n))$ & Physical routes that the segment list \\
% % 	&  sl translates to\\
% $\mathcal{S}_j$ & Spreading of the metric $j$\\
% $\Gamma_j$ & Largest possible distance to explore \\
% 	& on the most simple metric (Mi),\\
% 	& determining the size of our\\
% 	& data structures ($min(cj \times t, c0 \times \mathcal{S}_j)$)\\
% \bottomrule
% \end{tabular}
% \end{center}
\onecolumn
\section*{Appendix: Additional Results}

\section{Effects of Valuations and Constraints on Execution Times}

\subsection{Random Weights \& Metric Spreading}

\begin{figure}[ht]
\begin{subfigure}{.49\textwidth}
  \centering
  \includegraphics[width=.95\linewidth]{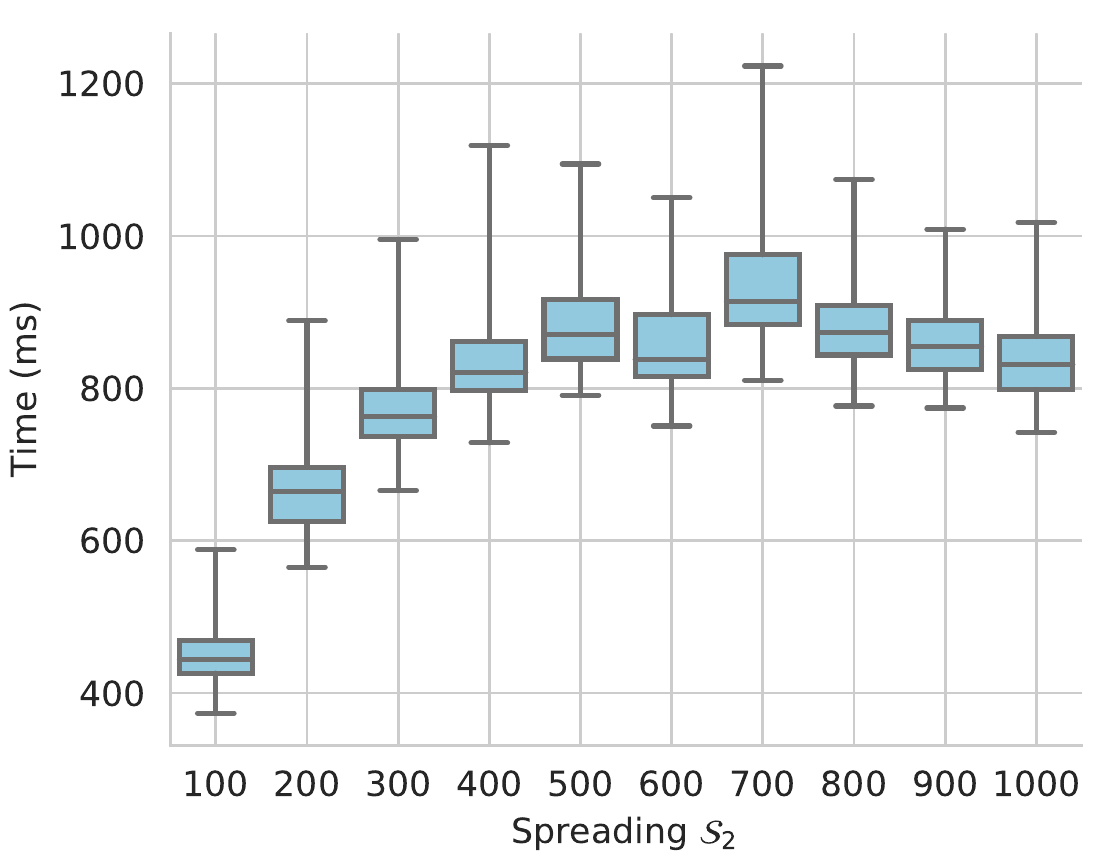}
  \caption{\bestcop performance on random SR graphs depending on $\mathcal{S}_2$.
  The execution times increase with $\mathcal{S}_2$, as our data structures fill up more quickly to store the fast growing pareto front.
  The effect of the distances being ignored can be seen starting at an $\mathcal{S}_2$ of 700.}\label{fig:app:ws}
\end{subfigure}
\hspace*{0.1cm}
\begin{subfigure}{.49\textwidth}
  \centering
  \includegraphics[width=.95\linewidth]{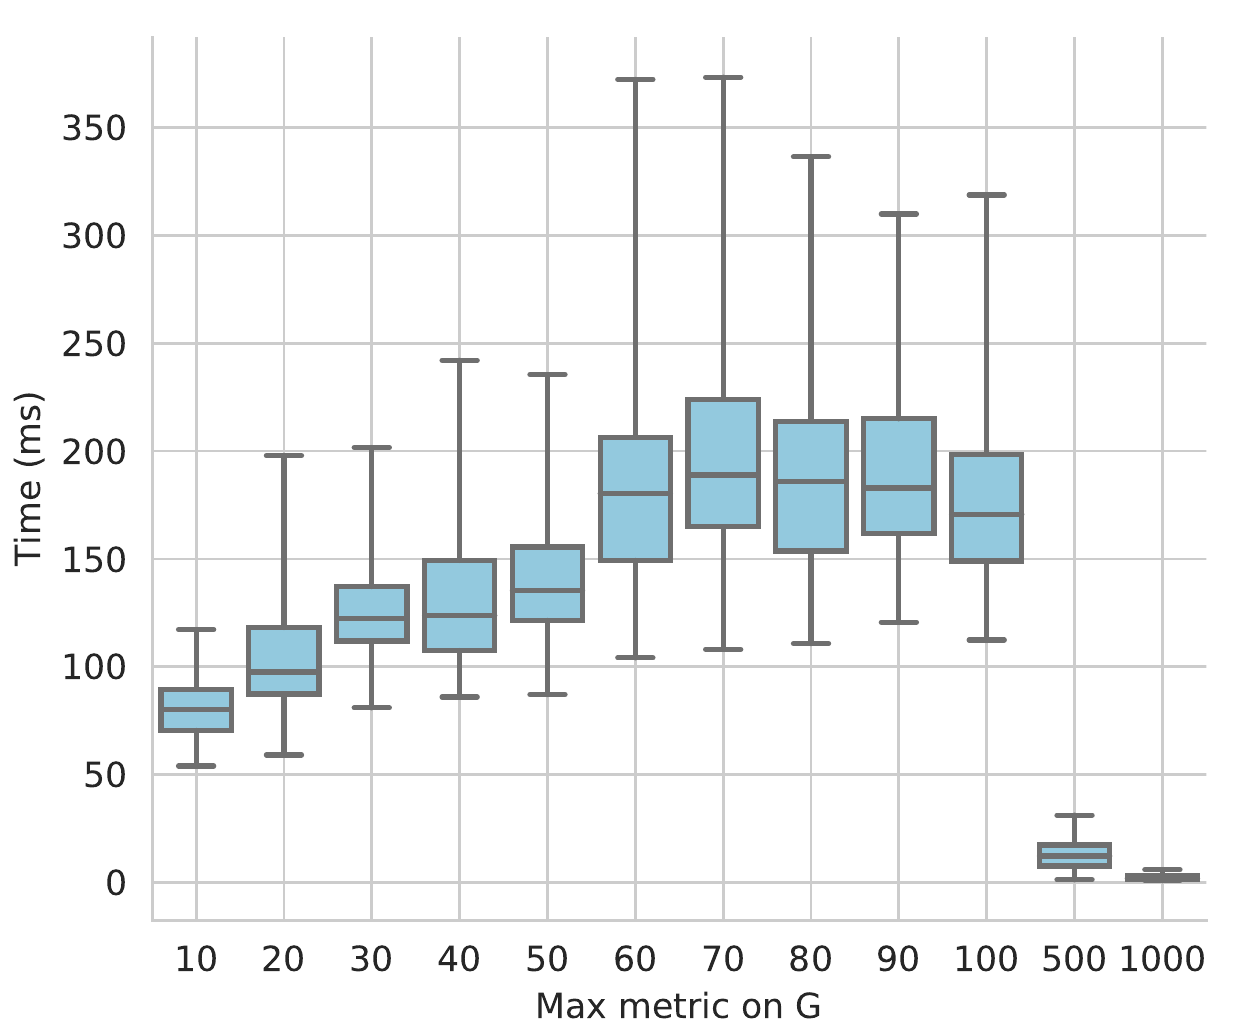}
  \caption{\bestcop performance on ISP-1 depending on the max weight in $E$
  (adding random M2 delays). The execution times increase with max metrics.
  However, past a certain point, the opportunity of ignoring paths with a distance above $\Gamma$ enhance the performances.}\label{fig:app:wss}
\end{subfigure}
\caption{The metric spreading affects the computing time.}
\end{figure}

Fig.~\ref{fig:app:ws} shows the impact of the spreading $\mathcal{S}_2$ on
\bestcop performance, on randomly weighted SR graph. We consider here the
maximum value of the weight in $E'$, the spreading (on the SR graph). The
execution time increases with $\mathcal{S}_2$ until reaching a peak at $700$ for
an average time of about $900$ms, before decreasing to $800$ms for a spread of
1000. Past this peak, the effects of exceeding our maximum constraint on $c2$
(1000) with the explored distances can be seen, as \bestcop executes slightlyIn summary, while, at first, more diverse weights fill up our data structure
quickly, this effect is then counterbalanced by the fact that we can ignore many
explored paths as their distances exceeds our by design constraint $c2=100ms$
(equivalent to $\Gamma = 1000$) -- because their distances increase as well as
the maximum weight.
faster.

Similarly to Fig.~\ref{fig:app:ws}, Fig.~\ref{fig:app:wss} shows the impact of
the maximum value of the weight, but this time in $E$ (the non-transformed
graph) on the execution time. That is what we call the pre-spreading. This
experiment was done on the ISP-1 topology and allowed us to extract the less
advantageous case for our experiments. We varied $s_2$ (the upper bound of the
random selection of the delay) from 10 to 1000, focusing on the range 10 to 100
in particular (because it decreases fast after). One can see that, at first, the
execution time increases with the max weight. As more values can appear on each
link, the number of collision on $M2$ diminishes as distances can now spread on
a larger interval. Thus, our structures, indexed on $M2$, fill up more quickly
with more paths to extend to guarantee the maintenance of the full pareto front,
leading to a higher execution time (from 75ms for $s_2=$ 10 to $\approx$ 200 for
$s_2=$ 70). However, after a certain point (namely, $s_2=$ 70), execution time
diminish. Indeed, as the maximum value of the weight rises, the number of paths
violating our maximum constraint $\Gamma = 1000$ increases as well, leading to
more and more pruned paths and thus better execution time (because nothing has
to be stored, and then extend, in our data structures).

In summary, while, at first, more diverse weights fill up our data structure
quickly, this effect is then counterbalanced by the fact that we can ignore many
explored paths as their distances exceeds our by design constraint $c2=100ms$
(equivalent to $\Gamma = 1000$) -- because their distances increase as well as
the maximum weight.

\subsection{Constraints \& Pruning}\label{sec:appendix:effect of constraints}

Up to now, all of the execution times shown did not rely on constraints stricter
than $c2=100ms$, and thus prevented us to prune paths during and even before the
execution to reduce the exploration space. However, in practice, ISPs would most
likely have strict constraints on delays, \eg $\approx 2$ to $20$ms, allowing
\bestcop to possibly ignore a large amount of paths that it would otherwise
explore.

\begin{figure}
\begin{subfigure}{.49\textwidth}
  \includegraphics[width=.95\linewidth]{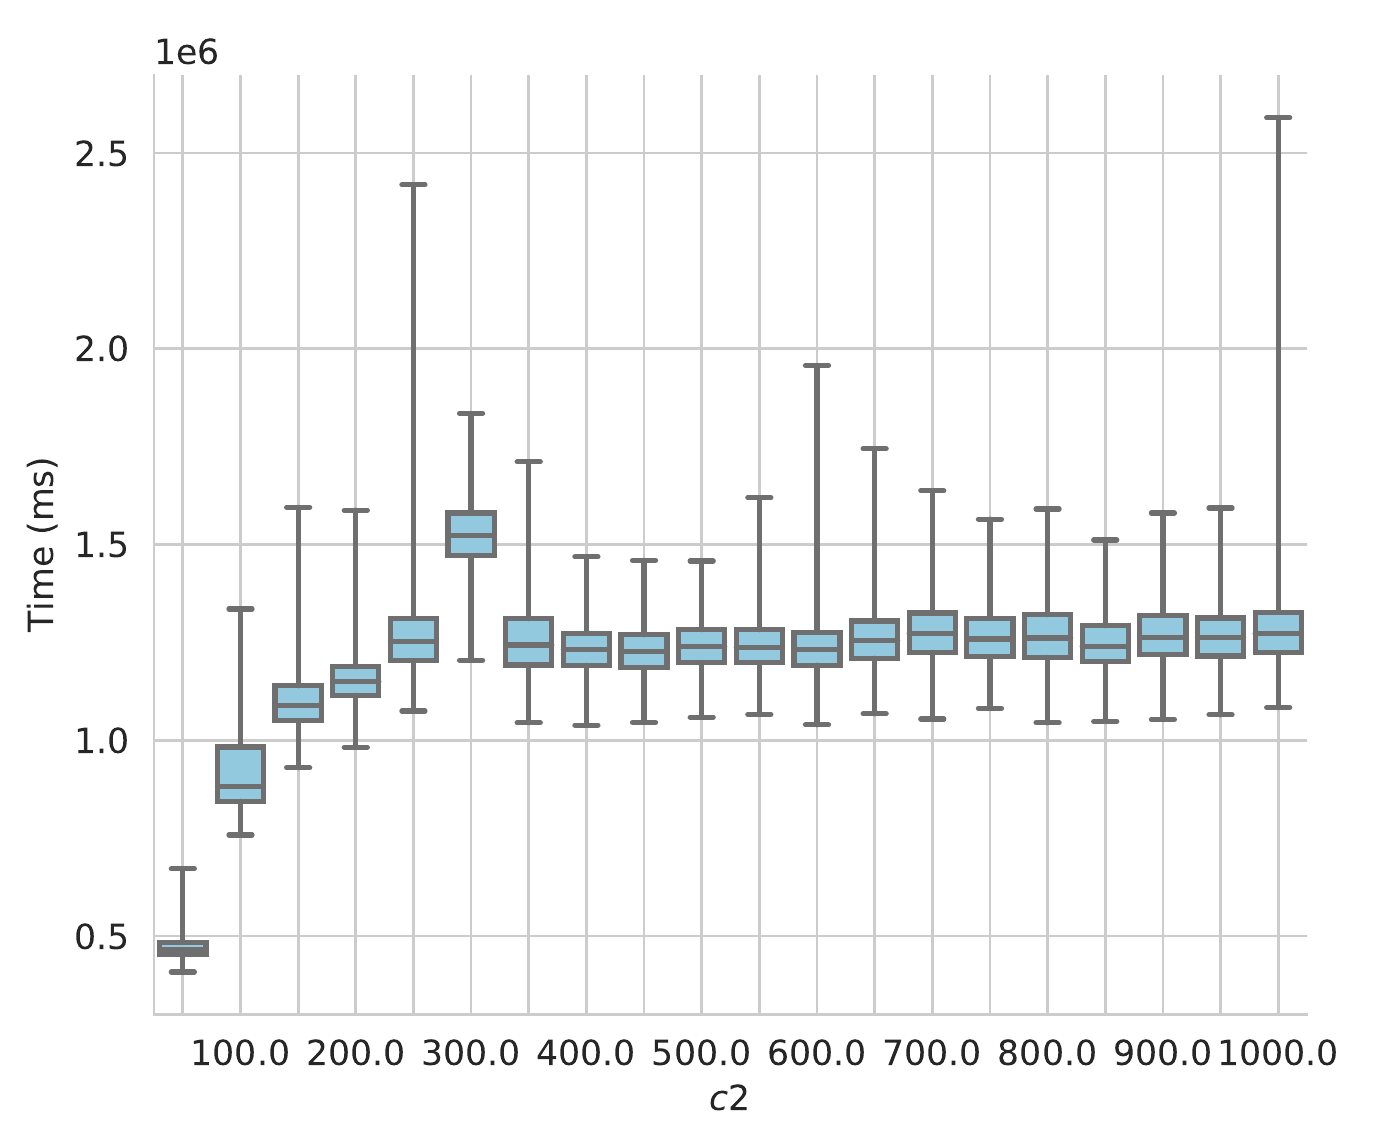}
  \caption{\bestcop execution time with respect to the constraint on $c2$, on a random SR graph. With $c2=100$, it means that we consider a constraint of 10ms. While very small constraints allows for pruning many paths and so reduces the execution time, when it exceeds 35ms, it looks to become stable.}
  \label{fig:eval:heatmap}
\end{subfigure}
\hspace*{0.1cm}
\begin{subfigure}{.49\textwidth}
  %\centering
  \includegraphics[width=.95\linewidth]{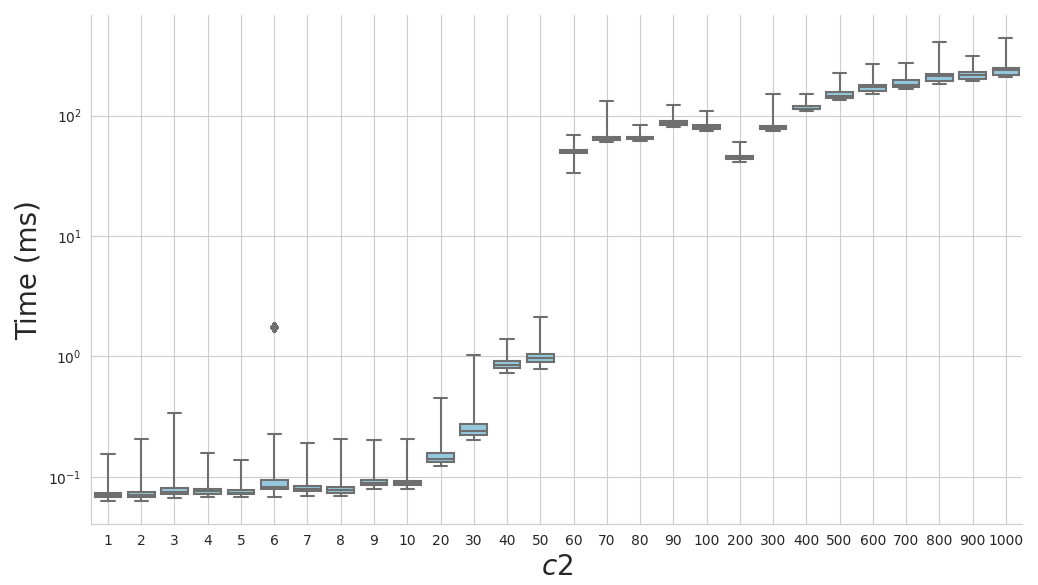}
  \caption{\bestcop execution time with respect to the constraint on $c2$, on ISP-1. Again, small constraints helps to save computing time. However, this effect tends to slow down when the saving enabled by the constraint reach a plateau. Finally, a great increase occur for value 6ms because feasible paths now exist and require to be extended.}
  \label{fig:eval:2fm}
  \end{subfigure}
\caption{Small constraints decreases the computing time.}
\end{figure}

Considering stricter constraints to be verified, \bestcop can perform even
better and so exhibits very good execution time to find constrained feasible
paths towards every other node. To conduct such an analysis, we first consider
the randomly valuated SR Graph that lead to the worst execution time in the
experiments described in Section~\ref{sec:2fm} (Figure~\ref{fig:eval:randfm}).
We then run \bestcop, adding a constraint $c2$ ranging from 0.1ms up to 100ms.
These results are shown in Fig.~\ref{fig:eval:heatmap}. We see that the ability
to prune path enhances our performances, lead to sub-millisecond execution time
for strict constraints. As the constraints grows larger, less paths are pruned
and the execution time increases. Once the constraint reaches a point where no
path can be pruned, the performance get stable. In practice, if we do not aim at
solving the 2COP optimization problem but rather the decision one (\ie 2CP), we
can expect execution times to drop as feasible paths get easier to find.
Fig.~\ref{fig:eval:2fm} provides the same kind of analysis but for the ISP-1
topology. Again we pick the specific one leading to worst computing times, \ie
with a pre-spreading of 70ms. The same effects are visible. Thanks to a finer
granularity, one can see that a gap is reached when enough feasible paths can be
extended to enable some real progression of the algorithm.

\section{Coverage \& Necessary Number of Segments for a Given M2 Constraint}
%\subsection{Playing with Constraints: Necessary Number of Segments}
\label{sec:constraints}

\begin{figure}[ht]
  \centering
  \includegraphics[scale=1]{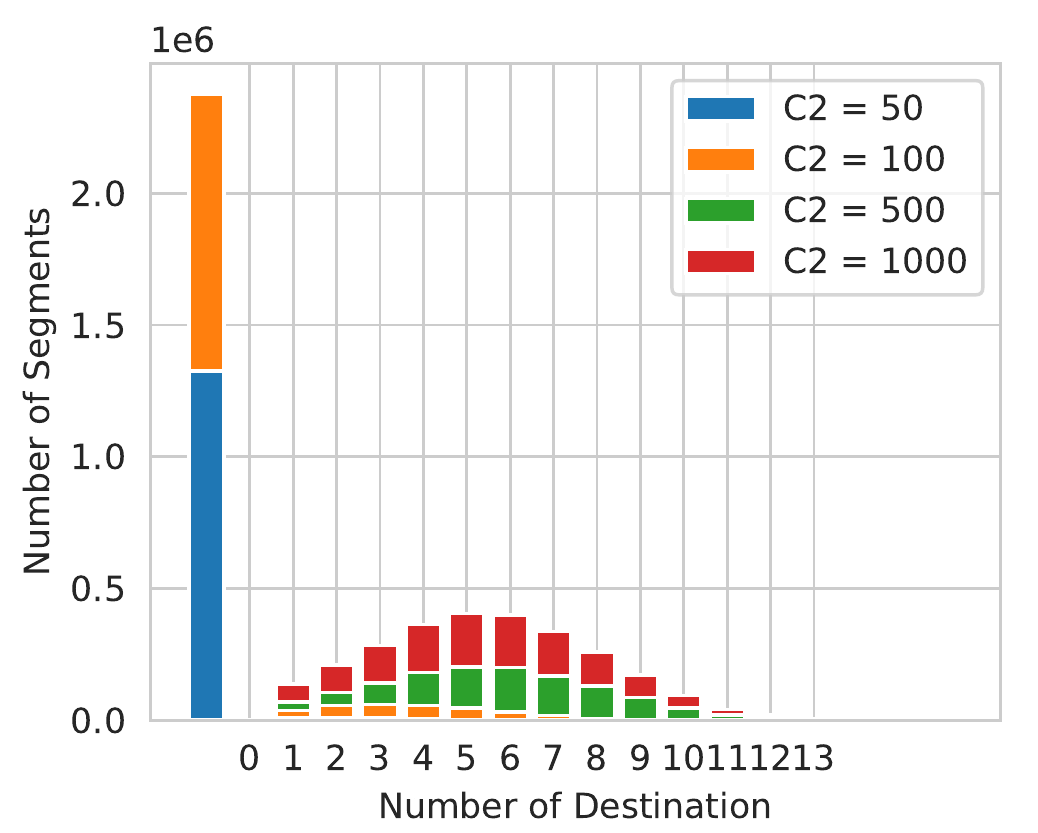}
  \caption{Distribution of the number of necessary TE segments depending on the source for our largest realistic topology on four constraints. It shows the minimal number of iterations to find every non-dominated paths towards a given node. While, for most destinations, every non-dominated path was listed before SEGMAX iteration, for some strict $c2$ constraints, it can require more than SEGMAX to claim the optimal exactitude.}
%  , some required more so the solution is not exact absolutely but almost.}
  % \bestcop is exact regarding $c0$.}
  \label{fig:eval:nb_iter}
\end{figure}

In this last section, we are interested in solving
$2COP+(\infty,\infty,1000,n),\forall n \in V$. For some constraints $c2' \leq
100 ms$ and for all $n \in V$, we then compare $woS(n) =
f(M1,\infty,\infty,c2',n)$ and $wS(n) = f(M1,10,\infty,c2',n)$. The first one
providing the optimal and so perfect overall answer (ignoring SEGMAX, $woS$)
while the second only output the best existing path under the SEGMAX constraint
(exact paths under all constraints, $wS$). Indeed, not considering SEGMAX as a
constraint (here $c0 = \infty$) enables us to understand how this constraint may
affect the coverage and reveal the inherent limitations of the router hardware
(making the SR architecture unable to use more than SEGMAX segments -- the
hardware limitation hampering its ability to copy more then SEGMAX at linerate).
By coverage, and for each destination $n$, we mean either that $ws(n) = woS(n)$
with $wS(n) \neq \emptyset$ (we call it \textit{perfect} coverage, \ie \bestcop
reach the optimality for $n$ despite the SEGMAX constraints), or $wS(n) \neq
woS(n)$ with $wS(n) \neq \emptyset$ (we call it \textit{imperfect} coverage, \ie
$wS(n)$ exhibits a path towards $n$ verifying $c2'$ but that is not optimal). On
the contrary, if $woS(n)$ is not empty while $wS(n)$ is, it means that the
SEGMAX constraint limits the ability of \bestcop to find a (M2) feasible path.
Finally, note that when $ws(n) = woS(n) = \emptyset$, it means that the
constraint is too strict to find a feasible path regardless of SEGMAX.

%TODO?
More formally, ...

Admittedly, we can only claim the exactness of \bestcop in a Segment Routing
context, as we do not explore paths that would require more than SEGMAX
segments. We only explore \textit{SR-feasible paths}
that respects $c0$, and thus may miss paths respecting $c2$ due to SR's operational constraints.
In this section, we explore the exactitude of \bestcop in the general case, putting SR aside.
In other words, we aim at studying if $c0$ is too restrictive when trying
to compute multi-constrained paths, \ie if SR \textit{hides} feasible solutions.
To do so, we do not stop the algorithm after SEGMAX iterations, but let it run until there is no path left to explore.
We keep, for each source the number of iterations (\ie the number of required segments) necessary to explore non-dominated path towards all other nodes.
We perform this evaluation on the real topologies studied in Section~\ref{sec:eval}. The results
are shown in Figures~\ref{fig:eval:nb_iter} for constraints of $5$, $10$, $50$, and $100$ ms.
The unlabel bar show destination for which no solution were found.

We can see that in many cases, a low number of segments is required, especially if the constraint is loose enough. Note that here we look for the optimal path that may require more segment hops than just a feasible one verifying the delay constraint.
We can relax that to only verify the $c2$ constraint and show that a path segment of less than SEGMAX exist in most situations and can show better performances.  In summary, in practice, once
constraints are loose enough to find paths, the latter will be found in almost always less than 10 iteration. However, a small minority are left unexplored.
